# Supplementary material for: BiHRNN -- Bi-Directional Hierarchical Recurrent Neural Network for Inflation Forecasting
Source: arXiv:2503.01893 source file (2025-02-27)
Supplement: Supplementary file 1 [file appendix.tex]

\chapter{Appendix title}

Appendix is just a different type of Section - it's included at the
end of the document (after the bibliography or list of references)
and before the Hebrew part and it's numbered in a different manner.
